# Supplementary material for: Automated Verification of Reactive and Concurrent Programs by Calculation
Source: arXiv:2007.13529 source file (2021-04-12)
Supplement: Supplementary file 1 [file appendix.tex]

In this appendix, we summarise our theory of reactive design contracts. The definitions are all mechanised in
accompanying Isabelle/HOL reports~\cite{Foster-RDES-UTP,Foster-SFRD-UTP}.

\subsection{Observational Variables}

We declare two sets $\tset$ and $\Sigma$ that denote the sets of traces and state spaces, respectively, and operators
$\tcat : \tset \to \tset \to \tset$ and $\tempty : \tset$. We require that $(\tset, \tcat, \tempty)$ forms a trace
algebra~\cite{Foster17b}, which is a form of cancellative monoid. Example models include $(\nat, +, 0)$ and
$(\seq\,A, \cat, \langle\rangle)$. We declare the following observational variables that are used in both our UTP
theories:
\begin{itemize}[]
  \item $ok, ok' : \Bool$ -- indicate divergence in the prior and present relation;
  \item $wait, wait' : \Bool$ -- indicate quiescence in the prior and present relation;
  \item $\state, \state' : \Sigma$ -- the initial and final state;
  \item $tr, tr' : \tset$ -- the trace of the prior and present relation.
\end{itemize}
Since the theory is extensible, we also allow further observational variables to be added, which are denoted by the
variables $r$ and $r'$.

\subsection{Healthiness Conditions}

We first describe the healthiness conditions of reactive relations.
\begin{definition}[Reactive Relation Healthiness Conditions]
\begin{align*}
  \healthy{R1}(P) & ~\defs~ P \land tr \le tr' \\
  \healthy{R2}_c(P) & ~\defs~ \conditional{P[\tempty, tr' \tminus tr/tr, tr']}{tr \le tr'}{P} \\
  \healthy{RR}(P) & ~\defs~ \exists (ok, ok', wait, wait') @ \healthy{R1}(\healthy{R2}_c(P))
\end{align*}
\end{definition}
$\healthy{RR}$ healthy relations do not refer to $ok$ or $wait$ and have a well-formed trace associated with them. The
latter is ensured by the reactive process healthiness conditions~\cite{Hoare&98,Cavalcanti&06,Foster17b}, $\healthy{R1}$
and $\healthy{R2}_c$, which justify the existence of the trace pseudo variable $\trace \defs tr' - tr$. $\healthy{RR}$
is closed under relational calculus operators $\false$, $\lor$, $\land$, and $\relsemi$, but not $\true$, $\neg$,
$\implies$, or $\II$. We therefore define healthy versions below.
\begin{definition}[Reactive Relation Operators]
\vspace{-1.2ex}

\begin{minipage}{.3\textwidth}
  \begin{align*}
    \truer  &~\defs~ \healthy{R1}(true) \\
    \negr P &~\defs~ \healthy{R1}(\neg P) \\
    P \rimplies Q &~\defs~ \negr P \lor Q
  \end{align*}
\end{minipage}
\begin{minipage}{.65\textwidth}
  \begin{align*}
    P \wpR Q &~\defs~ \negr (P \relsemi (\negr Q)) \\
    \IIr &~\defs~ (tr' = tr \land \state' = \state \land r' = r)
  \end{align*}
\end{minipage}
\end{definition}
We define a reactive complement $\negr P$, reactive implication $P \rimplies Q$, and reactive true $\truer$, which with
the other connectives give rise to a Boolean algebra~\cite{Foster17c}. We also define the reactive skip $\IIr$, which is
the unit of $\relsemi$, and the reactive weakest precondition operator $\wpR$. The latter is similar to the standard UTP
definition of weakest precondition~\cite{Hoare&98}, but uses the reactive complement.

We next define the healthiness conditions of reactive contracts.
\begin{definition}[Reactive Designs Healthiness Conditions]

\begin{minipage}{.2\textwidth}
\begin{align*}
  \healthy{R3}_h(P) & ~~\defs~~ \conditional{\IIsrd}{wait}{P} \\
  \healthy{RD1}(P) &~~\defs~~ ok \rimplies P \\
  \healthy{RD2}(P) &~~\defs~~ P \relsemi \ckey{J} \\
  \healthy{RD3}(P) &~~\defs~~ P \relsemi \IIsrd
\end{align*}
\end{minipage}
\begin{minipage}{.6\textwidth}
\begin{align*}
  \IIsrd            & ~~\defs~~ \healthy{RD1}(\conditional{(\exists \state @ \IIr)}{wait}{\IIr}) \\
  \healthy{R}_s     & ~~\defs~~  \healthy{R1} \circ \healthy{R2}_c \circ \healthy{R3}_h \\
  \healthy{SRD}(P) &~~\defs~~ \healthy{RD1} \circ \healthy{RD2} \circ \healthy{R}_s \\
  \healthy{NSRD}(P) &~~\defs~~ \healthy{RD1} \circ \healthy{RD3} \circ \healthy{R}_s
\end{align*}
\end{minipage}
\end{definition}
$\healthy{R3}_h$ states that if the predecessor is waiting then a reactive design behaves like $\IIsrd$, the reactive
design identity. $\healthy{RD1}$ is analagous to $\healthy{H1}$ from the theory of
designs~\cite{Hoare&98,Cavalcanti&06}, and introduces divergent behaviour: if the predecessor is divergent ($\neg ok$),
then a reactive design behaves like $\truer$ meaning that the only observation is that the trace is
extended. $\healthy{RD2}$ is identical to $\healthy{H2}$ from the theory of
designs~\cite{Hoare&98,Cavalcanti&06}. $\healthy{RD3}$ states that $\IIsrd$ is a right unit of sequential
composition. $\healthy{R}_s$ composes the reactive healthiness conditions and $\healthy{R3}_h$. We then finally have the
healthiness conditions for reactive designs: $\healthy{SRD}$ for ``stateful reactive designs'', and $\healthy{NSRD}$ for
``normal stateful reactive designs''.

Next we define the reactive contract operator.
\begin{definition}[Reactive Contracts]
  \begin{align*}
    \design{P}{Q} &~~\defs~~ (ok \land P) \implies (ok' \land Q) \\
    P \wcond Q    &~~\defs~~ \conditional{P}{wait'}{Q} \\
    \rc{\!P\!}{\!Q\!}{\!R}  &~~\defs~~ \ckey{R}_s(P \vdash Q \diamond R)
  \end{align*}
\end{definition}
A reactive contract is a ``reactive design''~\cite{Cavalcanti&06,Oliveira&09}. We construct a UTP design~\cite{Hoare&98}
using the design turnstile operator, $\design{P}{Q}$, and then apply $\healthy{R}_s$ to the resulting construction. The
postcondition of the underlying design is split into two cases for $wait'$ and $\neg wait'$, which indicate whether the
observation is quiescent, and correspond to the peri- or postcondition.

Finally, we define the healthiness conditions that specialise our theory to stateful-failure reactive designs.
\begin{definition}[Stateful-Failure Healthiness Conditions]
  \begin{align*}
    \Skip             &~~\defs~~ \rc{\truer}{\false}{\trace = \snil \land \state' = \state} \\
    \healthy{CSP3}(P) &~~\defs~~ \Skip \relsemi P \\
    \healthy{CSP4}(P) &~~\defs~~ P \relsemi \Skip \\
    \healthy{NCSP}(P) &~~\defs~~ \healthy{NSRD} \circ \healthy{CSP3} \circ \healthy{CSP4}
  \end{align*}
\end{definition}
$\Skip$ is similar to $\IIsrd$, but does not refer to $ref$ in the postcondition. If $P$ is $\healthy{CSP3}$ healthy
then it cannot refer to $ref$. If $P$ is $\healthy{CSP4}$ healthy then the postcondition cannot refer to $ref'$, but the
pericondition can: refusals are only observable when $P$ is quiescent~\cite{Hoare85,Cavalcanti&06}.
